# Supplementary material for: PhiNets: a scalable backbone for low-power AI at the edge
Source: arXiv:2110.00337 source file (2021-10-01)
Supplement: Supplementary file 1 [file appendix.tex]

\appendix

\section{Output of the pipeline}

A brief case study is here presented. Fig. \ref{fig:detresults_macc} shows some examples of results from the \texttt{MOT15} dataset. Let us suppose a situation akin the ones presented in the sequences \texttt{TownCentre}  (top-left in Fig \ref{fig:detresults_macc}) and \texttt{PETS09} (bottom-left), where a camera is mounted on an elevated position, overseeing a walkway.

\begin{figure}[h]
  \centering
  \includegraphics[scale=.25]{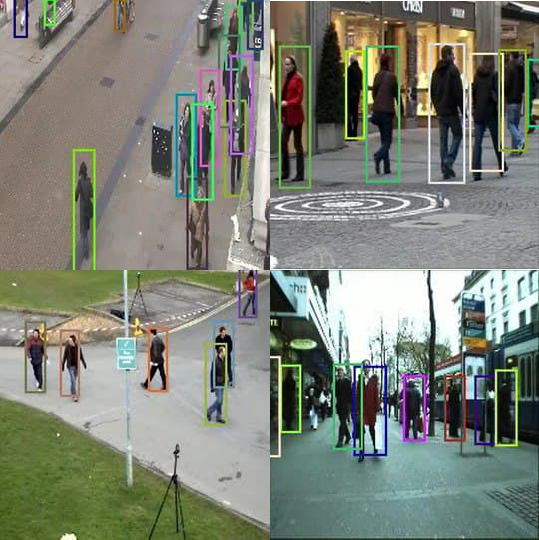}
  \caption{Visual example of detection and tracking pipeline's output.}
  \label{fig:detresults_macc}
\end{figure}

Situations like the ones presented are an ideal scenario for the proposed pipeline - a camera mounted on an elevated point means that there are no great variations in size and pose of the targets, allowing good tracking performance using smaller networks, with a low resulting power consumption. For example, the resulting MOTA score on \texttt{PETS09} is $62.86$ for the smallest network and $68.51$ for the largest one tested - the lighter network is very capable of generating good tracking results. Coupled with the fact that, given the large area seen by the camera, a relatively low fps can be used (targets will require multiple seconds to cross from one side of the image to the other), we can estimate the required energy usage for always-on tracking from Fig \ref{fig:average_power_fps}.\\
Given the target tracking accuracy, we can use the smallest tracking network presented in \ref{table:params}, at $3.18 MMACC$ complexity. Fig. \ref{fig:Inference_energy} shows the measured energy consumption per inference at $3.21 mJ$, or $16 mW$ at the chosen framerate. A similar result can be obtained from the plot in Fig. \ref{fig:average_power_fps}, knowing the target fps and noting that the network we are using is on the left side of the mAP bar.\\

Such low energy requirements are ideal for always-on IOT nodes, and in particular, a system with this kind of power consumption would have no problem running from even a really small solar panel - a typical $9cm \times 5cm$ monocrystalline solar panel can produce a peak power of around $913mW$
[ADD REF to datasheet], 
and assuming a conversion efficiency of $85\%$, a single hour under the sun could allow the system to run for 2 days uninterrupted.

NB: ho preso i dati dalla mia tesi (il pannello è quello comprato da digikey [ https://www.digikey.it/product-detail/it/anysolar-ltd/SM531K08L/SM531K08L-ND/9990469] e l'efficienza quella risultante dal caricabatterie che avevo progettato). Dobbiamo giustificare i valori in qualche modo? $85\%$ di efficienza non è fuori dal comune ma non saprei come giustificarla (potremmo mettere in ref il datsheet del convertitore utilizzato ma temo non lo vedano di buon occhio, dall'efficienza da datasheet a quella pratica di solito c'è un po' di divario)
